# Supplementary material for: SparseFed: Mitigating Model Poisoning Attacks in Federated Learning with Sparsification
Source: arXiv:2112.06274 source file (2021-12-12)
Supplement: Supplementary file 1 [file implicationsoftheory.tex]

\subsection{Practical Implications of Theory}
\label{appendix:theoryimplications}

We show the $\ell_2$ distances between the (counterfactual) benign and backdoored models in Table \ref{table:table-distances}. 
This realizes the improved bound in Theorem \ref{thm:main}, connecting our theory to practice. \algoname{} ensures the smallest distance to the benign model.

\begin{table}
\caption{Distances between the benign and backdoored models for various defenses. 
\algoname{} has the smallest distance as well as the lowest attack accuracy.}
\label{table:table-distances}

\centering 
\begin{tabular}{llll}
\toprule
\textbf{Defense} & \textbf{Distance ($\ell_2$)} & \textbf{Distance ($\ell_1$)} & \textbf{Attack acc}\\
 \toprule
%  & \textbf{CIFAR10} & & \textbf{CIFAR100} & & \textbf{FMNIST} & \\
 \textbf{FMNIST} \\
  \midrule
 Trimmed Mean & 51.4 & 95034 & 93.8\\
 Bulyan & 51.2 & 94772 & 84.6\\
 $\ell_2$ & 51.5 & 95554 & 100.0\\
 \textbf{\algoname{}} & 29.9 & 38935 & 2.4\\
  \midrule
%  \textbf{CIFAR10} \\
%  \midrule
%   Trimmed Mean & 69.5 & 43.2\\
%  Bulyan & 70.2 & 42.8\\
%  $\ell_2$ & 59.0 & 56.6\\
%  \textbf{\algoname{}} & 57.8 & 22.0\\
%  \midrule
%  \textbf{CIFAR100} \\
%   \midrule
%  Trimmed Mean & 184.2 & 45.8\\
%  Bulyan & 183.65 & 49.8\\
%  $\ell_2$ & 61.0 & 73.0\\
%  \textbf{\algoname{}} & 59.3 & 22.4\\
%  \midrule

% None & 106859 & 78.10 & 100 \\
% $\ell_2$ & 61099 & 0.7605 & 0.9700 \\
% \algoname{} & 31558 & 0.8142 & 0.0680 \\
% $\ell_2$ & 68259& 83.85 & 66 \\
% \algoname{} & 53354 & 81.72 & 24.4 \\
% \algoname{} (\fedssgd{}) & 172155 & 0.8280 & 0.0940 \\
\bottomrule
\end{tabular}
\vspace*{-10pt}
\end{table}
