# Supplementary material for: SparseFed: Mitigating Model Poisoning Attacks in Federated Learning with Sparsification
Source: arXiv:2112.06274 source file (2021-12-12)
Supplement: Supplementary file 2 [file certified.tex]

\vspace*{-13pt}
\section{Certified Robustness}\label{sec: empirical}
\vspace*{-2pt}
% \subsection{Certified Robustness}
We compute certified robustness guarantees for \algoname{} across MNIST, FashionMNIST, and CIFAR10, and compare to prior work~\citep{jia2020intrinsic, xie2021crfl, cao2021provably, levine2021deep}.
We report the \emph{certified accuracy}, which is the fraction of the test dataset for which (a) the model prediction is equal to the ground truth and (b) the distance between the top two model predictions is greater than the certified radius.

Because the threat model of \citep{xie2021crfl} only considers a single iteration of attack, we use their proposed procedure to extend their defense to fixed frequency attacks, which are the attacks in our threat model.
We first compute the total divergence by applying Theorem 2, and then use the total divergence in Theorem 3.
As we discuss in Section \ref{sec: related_work}, the defense in \citep{cao2021provably} cannot be scaled to the scale of $10,000$ clients, so we instead scale our setting down to $1000$ clients so that we can compare to their reported results.

Despite scaling down the setting, we still conduct experiments in the cross-device setting, i.e. data is not distributed i.i.d.\ across clients.
If results in the non-i.i.d.\ setting are unavailable \citep{jia2020intrinsic,cao2021provably,levine2021deep}, we compare results from the i.i.d.\ setting in those works.
Wherever code is not available (e.g. \citep{jia2020intrinsic, cao2021provably}) we estimate exact numbers from the provided figures.

In Table \ref{table:certified-mnist} we show certified accuracy on MNIST. 
We first train a single layer neural network on MNIST, with each of 1000 devices possessing 50 datapoints from 1 of the 10 classes, and 10 devices participating in each iteration.
% We use the output logits to generate the highest and second highest predicted probabilities for each datapoint in the test dataset.
% Naturally, more accurate models will have a larger gap between the top two probabilities, and therefore be more robust.
We compute the certified radius with Algo. \ref{alg:radius} and the certification with Algo. \ref{alg:certify}.
For a very small percentage of attackers, our defense is comparable to prior work.
However, as the percentage of attackers increases, our defense rapidly stands head and shoulders above all prior work.


\begin{table}
  \caption{\algoname{} surpasses prior work in certified accuracy on MNIST, across varying numbers of attackers}
  \label{table:certified-mnist}
  \centering
  \begin{tabular}{llllll}
    \toprule
    % \multicolumn{2}{c}{Certified Accuracy on MNIST ($\%$ Poisoned)}                   \\
    % \cmidrule(r){1-2}
    Name   &  0.1 & 1 & 2 & 4 & 8 \\
    \midrule
    \citep{xie2021crfl} & 47.08 & 0 & 0 & 0 & 0 \\
    \citep{jia2020intrinsic} & 80 & 50 & 5 & 0 & 0 \\
    \citep{levine2021deep} & 88 & 0 & 0 & 0 & 0 \\
    \citep{cao2021provably} & 88 & 83 & 72 & 40 & 0 \\
    \textbf{SparseFed (Ours)} & 88.16 & 88.16 & 87.40 & 73.13 & 73.36 \\
    \bottomrule
  \end{tabular}
\end{table}

\begin{table}
  \caption{}
  \label{table:certified-cifar}
  \centering
  \begin{tabular}{lllll}
    \toprule
    \multicolumn{2}{c}{Certified Robustness on CIFAR10 ($\%$ Poisoned)}                   \\
    \cmidrule(r){1-2}
    Name     & 1 & 2 & 4 & 8 \\
    \midrule
    \citep{xie2021crfl} \\
    \citep{jia2020intrinsic}  \\
    \textbf{SparseFed (Ours)} & 24.05 & 22.30 & 18.75 & 13.01 \\
    \bottomrule
  \end{tabular}
\end{table}
