# Supplementary material for: SparseFed: Mitigating Model Poisoning Attacks in Federated Learning with Sparsification
Source: arXiv:2112.06274 source file (2021-12-12)
Supplement: Supplementary file 3 [file connecting_model_robustness_to_adversarial_accuracy.tex]

\section{Certifiable malicious accuracy from model robustness}\label{appendix:certif}

In this section, we connect malicious accuracy to model robustness.

\begin{definition}[Loss Lipschitzness with respect to model parameters.]
For a loss function $\ell$ and a data point $x$ and a set of models $\Theta$ , we define the loss lipschitzness  of loss function $\ell$ with respect to model parameters and for point $x$ to be,
$$c_{\ell,x,\Theta} = \inf_{\theta_1\neq \theta_2\in \Theta} \frac{\ell(\theta_1,x)-\ell(\theta_2,x))}{|\theta_1-\theta_2|}.$$
Also, for a set of inputs $X$ we define 
$c_{\ell,X,\Theta} = \sup_{x\in X} c_{\ell,x,\Theta}.$
\end{definition}
\begin{remark}
The definition above is a composition of Lipschitzness of the model output with respect to its parameters and the Lipschitzness of the loss function with respect to its input. Specifically, if the model on a point $x$ is $c_1$ lipschitz with respect to its parameters, and the loss is $c_2$ lipschitz, then $c_{\ell,x,\Theta} \leq c_1\cdot c_2$.
\end{remark}
\begin{definition}[Federated Learning with Robust Model Weights]
A federated learning protocol $L=(f,A)$ has $(\alpha,\epsilon)$-robust model weights if for any set of benign agents $S_b$ and any set of malicious agents $S_m$,  it has the guarantee that 
$$\Pr_{r\gets \mathcal{R}}\Big[|L(S_b \cup S_m,r) - L(S_b,r)| \leq \alpha(|S_m|,|S_b|)\Big]\geq 1-\epsilon(|S_m|,|S_b|)$$
\end{definition}

\begin{theorem}
Let $L=(f,A)$ be a federated learning protocol that has $(\alpha,\epsilon)$-robust model weights that output a model from a set of models $\Theta$. Then, for any set of malicious and benign agents $S_b$ and $S_m$, for any loss function $\ell$, any point $x$ and any constant $\eta$ we have,

$$\Pr_{M\gets L(S_b \cup S_m)}\big[\ell(M,x)\leq \eta\big] \geq \Pr_{M\gets L(S_b)}\big[\ell(M,x)\leq \eta - c_{\ell,x,\Theta}\cdot \alpha(|S_m|,|S_b|)\big] -\epsilon(|S_m|,|S_b|).$$
\end{theorem}

\begin{proof}
Let $M=L(S_b,r)$ for some randomness $r$. Also, let $M'=L(S_m\cup S_b,r)$ for the same randomness $r$. If $\ell(M',x)> \eta $
Then by lipschitzness of the loss with respect to model parameters we have that
$\ell(M,x)\geq \eta - c_{\ell,x,\Theta}|M-M'|.$
Therefore we have,
$$\Pr[\ell(M',x)> \eta ]\leq \Pr[\ell(M,x)> \eta - c_{\ell,x,\Theta}|M-M'|].$$
On the other hand, we know that $\Pr[|M-M'| \geq \alpha(|S_m|,|S_b|)]\leq \epsilon(|S_m|,|S_b|)$. Therefore we have
$$\Pr[\ell(M',x)> \eta ]\leq \Pr[\ell(M,x)> \eta - c_{\ell,x,\Theta}\cdot\alpha(|S_m|,|S_b|)] + \epsilon(|S_m|,|S_b|).$$
Then, negating the inequality and adding 1 to both sides proves the statement of theorem. 
\end{proof}
