# Supplementary material for: SparseFed: Mitigating Model Poisoning Attacks in Federated Learning with Sparsification
Source: arXiv:2112.06274 source file (2021-12-12)
Supplement: Supplementary file 4 [file old_theory.tex]

\vspace*{-13pt}
\section{Theoretical Analysis}
% \vspace*{-2pt}
\label{appendix:theory}
\begin{definition}
% \vspace*{-5pt}


For a parameter $1 \leq k \leq d$, the operator $top_k$: $\mathbb{R}^d \rightarrow \mathbb{R}^d$ is defined for $x \in \mathbb{R}^d$ as
% \begin{center}
%\vspace*{-5pt}
% \begin{align}
$
    (\text{top-}k(x))_i \coloneqq \begin{cases}
    (x)_\pi(i) & \text{if $i \leq k$}\\
    0 & \text{otherwise}
    \end{cases}
    $
    
% \end{align}
% \end{center}
where $\pi$ is a permutation of $[d]$ such that $(|x|)_{\pi}(i) \geq (|x|)_{\pi}(i+1)$ for $i=1,..., d-1$. 
\end{definition}
\vspace*{-5pt}

\paragraph{Robustness of norm clipping:}
We begin by analyzing the $\ell_2$ clipping component of \algoname{} in isolation without top-$k$, and see that we need further defenses to mitigate the model poisoning attack.
% \prateek{should we rephrase this text to highlight that we are analyzing the norm clipping component of our defense in isolation here, without top-k?}
% Our key insight is to combine global top-$k$ update sparsification with norm clipping as a defense mechanism.
We aim to calculate an upper bound on the distance between attacked and unattacked models trained with federated learning.
% Federated learning consists of multiple rounds; at each round, a a subset of devices sends an update that is taken with respect to the current model, that is the summary of the protocol so far.
% As we mention in Section \ref{sec: related_work}, making updates differentially private can mitigate the impact of attackers.
% Because boosting is typically necessary in order to ensure the attacker can insert their backdoor, $\ell_2$ norm clipping introduces robustness by diminishing the effect of boosting.
% Afterwards, a Lipschitz mechanism such as uniform averaging combines the gradients and updates the model.
We first bound the update of iteration $i$ for a federated learning system that implements $\ell_2$ clipping of norm $L$ as:
\[|u^i-u^i_b|_1 \leq \sqrt{d}L\cdot p.\]
where $u^i$ is the gradient aggregated over all users, $u^i_b$ is the gradient aggregated over only benign parties, and $p$ is the fraction of attackers in the population.
If the protocol only has 1 round where attackers may be present, norm clipping will be sufficient to mitigate their effects.
However, the protocol has multiple adaptive rounds, and any small change in iteration $i$ can propagate and lead to large changes in the next iterations.
To handle this propagation error, we need to bound the effect that changes in previous rounds have on the gradients of future rounds. 
This is where we employ our Lipschitzness guarantees. 
We prove the following informal theorem that uses the Lipschitz continuity of the gradients:
\begin{theorem}[Robustness of $L_2$ norm clipping]\label{thm:inf1}
For a protocol with $c$-Lipschitz coordinate-wise gradients, using $\ell_2$ norm clipping with threshold $L$ and decreasing learning rate $\frac{\alpha}{i}$ we have
%\vspace*{-10pt}
$$|M^T -M^T_b|_1\leq \tilde{O}(\alpha T^{\alpha d c}Lp\sqrt{d})$$
where $d$ is the dimension of the model $M$, $p$ is the fraction of corrupted devices, $M^T$ is the model obtained after $T$ iterations and $M^T_b$ is the model after $T$ iterations using only benign devices.
\end{theorem}

\paragraph{Robustness of \algoname{}:} In practice $d$ is large, therefore $\ell_2$ clipping is insufficient to mitigate attacks.
We confirm this analysis with our experiments in Section \ref{sec: evaluation}.
Next we show that the combination of gradient sparsification and $\ell_2$ clipping can alleviate the curse of dimensionality, and obtain better robustness guarantees.
% \begin{definition}[ $top_k$ with memory and $\gamma_k$]\label{def:gamma}
% We can apply the $top_k$ operator to any aggregator $A$ to obtain a new aggregator $A^k$: $A^k$ initializes a memory vector $W_0=0^d$ and an initialization $M_0$.
% At step $i$, $A^k$ receives the update $u^1,\dots,u^n$ and calculates the $top_k$ $I=\set{i\in [d]; top_k(W_{i-1}+\sum_{j=1}^nu^j)\neq 0}$.
% Then, the memory and model are updated:
% %\vspace*{-5pt} % ICML
% {\begin{small}
% \begin{align}
% W_i = W_{i-1} +\sum_{j=1}^nu^j - top_k(W_{i-1}+\sum_{j=1}^n(u^j))
% M_i=A_i(M_{i-1}, (u^1)_I,\dots,(u^n)_I) 
% \end{align}
% \end{small}}
% %\vspace*{-2pt} % ICML
% where $(u)_I$ is a vector that is $0$ everywhere except on coordinates $i\in I$ where it is equal to $u$.
% We also define $\gamma_k$ to be the fraction of $l_1$ mass of information lost via $top_k$.
% Specifically, for any model $M$, any $i\in [T]$ and update vector $(u^1,\dots,u^n)$ calculated by all parties (including attackers), and memory $W$, we have:
% %\vspace*{-10pt} % ICML
% \begin{align}
%     |top_k(\sum_{j=1}^n u^j + W)|_1\geq (1-\gamma_k)|\sum_{j=1}^n u^j +W|_1.
% \end{align}
% %\vspace*{-2pt} % ICML
% When clear from the context, we use $\gamma$ instead of $\gamma_k$. Note that $\gamma_k$ can be a function of the distribution of the updates and $k$. 
% For example, if the updates are concentrated on a small number of coordinates, we expect $top_k$ to recover nearly the entire mass and $\gamma_k$ to be small. 
% \end{definition}

\begin{theorem}\label{thm:main}
Let $(f,A)$ be a $(c_1,c_2)$-Lipschitz protocol such that $f_i$ uses a learning rate of $\alpha_i$.
Let $A^{L,k}$ be the the same aggregator as $A$ but equipped with $\ell_2$-norm clipping and with a clipping threshold of $L$, and the $top_k$ operator. 
Let $M_b$ be the model obtained by learning using the set of benign devices $S_b$, and $M$ be the model obtained by learning using all devices (including attackers) in $T$ iterations using the protocol $(f,A^{L,K})$. 
Then we have:
%\vspace*{-5pt} % ICML
$$|M^T -M^T_b|_1\leq \tilde{O}(\alpha T^{\alpha k c}L\sqrt{d}(p + \gamma_k)).$$
%\vspace*{-20pt} % ICML
\end{theorem}
% Before proving Theorem \ref{thm:main}, we state a Corollary that simplifies this bound. 
% \begin{corollary}\label{cor:inf}
% Simplifying the bound of Theorem \ref{thm:main} we get

% \end{corollary}

Comparing Theorem \ref{thm:main} above with Theorem \ref{thm:inf1}, we see that we have improved the exponent of $T$ from $cd$ to $ck$.
$cd$ is the Lipschitz constant of the model when $top_k$ is not deployed, which we reduce it to $ck$ by using $top_k$ operator.
This bound on how far the attacker can shift the model acts as an additional constraint on the attacker, that can only improve security.
In Appendix B.6 we confirm that reducing the distance improves robustness.

This improvement does not come for free. 
In general, $\gamma_k$ is an decreasing function of $k$, however, our experiments show that we can obtain very small values of $\gamma_k$ with $k<<d$. 
Another important consideration is the number of iterations.
When $k$ is very small, we expect the number of iterations required for convergence to increase. 
To optimize this trade-off, in Section \ref{sec: evaluation} we find small values of $k$ that provide us with strong robustness.

\emph{In summary, our \algoname{} protocol  aggregates $\ell_2$ clipped gradients from devices and only updates the top-$k$ coordinates of the aggregated gradient.
We show that the use of top-$k$ update sparsification upper bounds the distance that an attacker can shift the model over the course of training.}

% \prateek{it could be useful to have a summary sentence about our proposed defense (update sparsification/norm clipping) + another one on the L2 distance bound Ashwinee: How's this?}

% \begin{proof}[Proof of Theorem \ref{thm:main}]
% We define two sequences of models $(M_b^0, \dots, M_b^T)$ and $(M^0, \dots, M^T)$ where $M_b^i$ is the model trained in the first $i$ iterations from the data of devices in  $S_b$ and $M^i$ is the model trained in the first $i$ iterations for all devices.
% We prove Theorem \ref{thm:main} with a series of Lemmas.
% Let $W^i$ be the memory of $top_k$ at iteration $i$ and $W^i_b$ be the memory when only the gradients of the benign devices are used up to iteration $i$. 
% Let $u$ be the summation of update vectors of all devices on $M^{i-1}$ and $u_b$ the summation of update vectors of benign devices in $S_b$ over $M^{i-1}_b$. 
% We first want to bound
% $$|top_k(\frac{u_b}{|S_b|} + W_b^{i-1}) - top_k(\frac{u}{|S|} + W^{i-1})|.$$

% We first state the following claim
% that shows a recursive relationship for the distance between the benign and adversarial models. 
% The proof of this claim is deferred to the Appendix.
% \begin{claim}\label{clm:recursive}
% We have
% \begin{align*}
% |M^i - M^i_{b}|_1&\leq|M^{i-1} - M_b^{i-1}|(1 + \frac{2kc_1c_2}{i} )\\
%  &~~~+ L\sqrt{d}(\frac{c_1|S\setminus S_b|}{i|S|} +\frac{4c_1 \gamma }{i\cdot (1-\gamma)}).
% % \stepcounter{equation}\tag{\theequation}\label{eq:006}
% \end{align*}
% \end{claim}
% The inequality of Claim \ref{clm:recursive} shows a recursive relation between $|M^i - M^i_b|$ and $|M^{i-1}  - M^{i-1}_b|$. The following lemma shows how we can use this recursive relationship to bound the distance.
% \begin{lemma}\label{lem:recursive}
% Let $S_{\N}$ be a sequence such that $S_0=0$ 
% $$S_{i} \leq (1+\frac{A}{i})S_{i-1} + \frac{B}{i}$$
% then for any $T$ we have
% $$S_T \leq (1+\ln(T))\cdot {(A+1)^{\ln(T)}}\cdot B.$$
% \end{lemma}
% Now using the recursive relation of Claim \ref{clm:recursive} and using the fact that $|M^0-M_b^0|=0$ and deploying Lemma \ref{lem:recursive} we get
% \begin{align*}&|M^{T} - M_b^{T}|\leq\\
% &c_1L\sqrt{d}(1+\ln(T)) \cdot (2+ 4k c_1 c_2)^ {\ln(T)}(\frac{|S\setminus S_b|}{|S|} + \frac{2\gamma}{1-\gamma} )
% \end{align*}
% which finishes the proof.
% \end{proof}

% Federated learning is a protocol consisting of $n$ parties $P_1,\dots,P_n$ and a central aggregator $G$. 
\begin{definition}[Federated Learning Protocol] Considering a federated learning protocol with $n$ clients $P_1,\dots,P_n$.
Let $Z$ be the data domain and ${\cP_i}_{i=1}^{n}$ be $n$ probability distributions over $Z$.
The $i^{th}$ client has a dataset $D_i$ drawn i.i.d. from $\cP_i$.
% Let $\cM$ be the class of models in $d$ dimensions, and $\cL: \cM \times Z \rightarrow \cR$ be a loss function.
% Our goal is to minimize the empirical risk:
% \begin{align}
%     f(\M) = \hat{\mathbb{E}}f_i(\M) =
%     \frac{1}{n}\sum_{i=1}^n \Eu{\z \sim \cP_i}\cL(\M,\z).
% \end{align}
We conduct $T$ rounds of the protocol, and at round $i\in[T]$ each participating client downloads the current model $M_{i-1}$.
% Each $P_i$ has a dataset $D_i$. The aggregator $G$ holds an initial model $M_0$. The protocol consists of $T$ rounds and at round $i\in [T]$, the aggregator sends $M_{i-1}$ to all parties. 
% Each of them calculate a (potentially randomized) function $f_i$ on their data
% $$u^j_i=f_i(M_{i-1}, D_j)$$
% and send it back to the aggregator. Then the aggregator applies a function $A$ to aggregate all the updates

% $$M_i=A_i(M_{i-1}, u_i^1,\dots,u^n_i).$$

% For instance, if the goal of this protocol is to train a network using SGD with simple averaging aggregation, then 
For example, one common instantiation of a federated learning protocol is the following: Each client calculates the result of gradient descent $f_i$ on its data:

$$f_i(\M, D) =  \frac{\partial \cL(\M,D)}{\partial \M}$$

And the parameter server averages the updates across participating clients:

$$A_i(M_{i-1}, u_i^1,\dots,u^n_i) = M_{i-1} + \frac{1}{n}\sum_{j=1}^n u_i^j$$
\end{definition}
%  where $\beta_i$ could be seen as the decaying learning rate and is usually set to $\frac{\alpha}{i}$ for some constant $\alpha$.
\begin{definition}[Lipschitz Federated Learning] A federated learning protocol is $(c_1,c_2)$-Lipschitz if for any round $i\in[T]$, any two models $M_1, M_2\in \cM$, any two sequences of update vectors $(u^1,\dots,u^n)$ and $(u'^1,\dots,u'^m)$, and any dataset $D$ we have
$$|f_i(M_2,D)-f_i(M_1,D)|_\infty \leq c_1\cdot |M_2-M_1|_1$$
and 
\begin{align*}
    &|A_i(M_1, u^1,\dots,u^n) - A_i(M_2,u'^1,\dots,u'^m)|_1\leq |M_1-M_2|_1 + \frac{c_2}{i}(|\frac{\sum_{j=1}^{n}u^j}{n}-\frac{\sum_{j=1}^{m}u'^j}{m}|_1)
\end{align*}
\end{definition}

\begin{definition}\label{def:gamma}[$\gamma_k$ for top-$k$ operator]
Let $\gamma_k$ be the fraction of $l_1$ mass of information lost via $top_k$, where $top_k(u)$ recovers a $1-\gamma_k$ fraction of the $l_1$ mass of $u$.
% In particular, $1-\gamma_k$ fraction of the $l_1$-norm mass of the gradients should be recovered after top-$k$ is applied. 
For any model $M$, any $i\in [T]$ and update vector $(u^1,\dots,u^n)$ calculated by all parties (including benign and adversarial gradients), and memory $W$, we have:
\begin{align}
    |top_k(\sum_{j=1}^n u^j + W)|_1\geq (1-\gamma_k)|\sum_{j=1}^n u^j +W|_1.
\end{align}
When clear from the context, we use $\gamma$ instead of $\gamma_k$.
\end{definition}
Now we prove the following general Theorem that we use to prove Theorems \ref{thm:inf1} and \ref{thm:main}.
\begin{theorem}\label{thm:main2}
Let $(f,A)$ be a $(c_1,c_2)$-Lipschitz protocol such that $f_i$ uses a learning rate of $\alpha_i$.
Let $A_{L,k}$ be the aggregator that conducts an average, equipped with $l_1$-norm clipping with a clipping threshold of $L$, and the top-$k$ operator. 
Let $M_b$ be the model obtained by learning using the set of benign agents $S_b$, and $M$ be the model obtained by learning using all agents (benign and adversarial) in $T$ iterations using the protocol $(f,A_{L,K})$. 
Then we have:

\begin{align*}&|M^{T} - M_b^{T}|_1\leq2c_1L(1+\ln(T)) \cdot (1+ 2k c_1 c_2)^ {\ln(T)}(\frac{|S\setminus S_b|}{|S|} + \frac{2\gamma}{1-\gamma} =\tilde{O}(\alpha T^{2k c_1c_2}L\sqrt{d}(p + \gamma_k)).)
\end{align*}
\end{theorem}
\begin{proof}
We first define two sequence of model $(M_b^0, \dots, M_b^T)$ and $(M^0, \dots, M^T)$ where $M_b^i$ is the model trained in the first $i$ iterations from the data of the agents in  $S_b$ and $M^i$ is the model trained in the first $i$ iterations for all agents.  We prove the Theorem by using a series of Lemmas.
% First note that $M_b^0=M^0$ as the first element of the sequence is just the random initialization and is the same for both sequences. Now we make this strong induction hypothesis: At each iteration $i$, we have
% \begin{equation}|W_b^i-W^{i}|+|M^i_b-M^i|_1\leq (1+c_1+c_2)\cdot k \cdot i \cdot L\cdot(\gamma + \frac{|S\setminusS_b|}{|S|})\end{equation}
Let $W^i$ be the ``memory'' of the top-$k$ at iteration $i$ and $W^i_b$ be the memory when only the gradients of the benign agents are used up to iteration $i$. 
% Note that the hypothesis is correct for $i=0$. Now assume we assume the hypothesis for $i-1$ and prove it for $i$. Assume we have
% \begin{equation}|W_b^{i-1}-W^{i-1}|+|M^i_b-M^i|_1\leq (1+c_1+c_2)\cdot k \cdot (i-1) \cdot L\cdot(\gamma + \frac{|S\setminusS_b|}{|S|}).\end{equation}

Let $u$ be the summation of update vectors of all agents on $M^{i-1}$ and $u_b$ the summation of update vector of benign agents in $S_b$ over $M^{i-1}_b$. We first want to bound
$$|top_k(\frac{u_b}{|S_b|} + W_b^{i-1}) - top_k(\frac{u}{|S|} + W^{i-1})|.$$

For that, we first prove the following two Lemmas whose proofs are deferred to appendix. 

\begin{lemma}\label{lem:topk}
Let $u_1$ and $u_2$ be two vectors in $\mathbb{R}^d$ such that $|top_k(u_1)|\geq(1-\gamma)\cdot |u_1|$ and  $|top_k(u_2)|\geq(1-\gamma)\cdot |u_2|$, then, for any vector $v$ we have
\begin{align*}
    &|top_k(u_1)-top_k(u_2)|_1 \leq |(u_1-u_2)_I|_1 + 2\gamma |u_2|_1 + 2\gamma |u_1|_1 
\end{align*}
where $I=\set{j\in [d] \text{~s.t.~} top_k(u_1)[j]\neq 0 \text{~or~}  top_k(u_2)[j]\neq 0}$.

\end{lemma}

\begin{proof}
Let $\tau_1$ and $\tau_2$ be two vectors such that $\tau_1[i]=1$ if $top_k(u_1)[i]\neq0$ and $\tau_1[i]=0$ otherwise. Similarly, $\tau_2[i]=1$ if $top_k(u_2)[i]\neq0$ and  $\tau_2[i]=0$ otherwise. Let $I'$ be the locations where $\tau_1[i]=1$ and $\tau_2[i]=1$. Now we have

\begin{align*}
    |top_k(u_1) -top_k(u_2)|
    &= \sum_{i=1}^d |u_1[i]\tau_1[i] - u_2[i]\tau_2[i]| \\
    &= |(u_1-u_2)_{I'}|_1 + \sum_{i\in I\setminus I' } |u_1[i]\tau_1[i] - u_2[i]\tau_2[i]|\\
    &\leq |(u_1-u_2)_{I'}|_1 + \sum_{i \in I\setminus I' } |u_1[i]\tau_1[i] - u_2[i]\tau_1[i]|\\
    &~~+\sum_{i \in I\setminus I' }|u_1[i]\tau_2[i] - u_2[i]\tau_2[i]|+ \sum_{i \in I\setminus I' }|u_2[i]\tau_1[i] - u_1[i]\tau_2[i] |\\
    &= |(u_1-u_2)_I|_1+ \sum_{i \in I\setminus I' }|u_2[i]\tau_1[i] - u_1[i]\tau_2[i] |\\
    &\leq |(u_1-u_2)_I|_1 + \sum_{i\in I\setminus I' } |u_1[i]\tau_2[i]| + |u_2[i]\tau_1[i]|\\
    &= |(u_1-u_2)_I|_1 + \sum_{i\in I\setminus I' } |u_1[i](1-\tau_1[i])|+ \sum_{i\in I\setminus I' } |u_2[i](1-\tau_2[i])|\\
    &\leq |(u_1-u_2)_I|_1 +  |u_1 -top_k(u_1)| + |u_2-top_k(u_2)|\\
    &\leq |(u_1-u_2)_I|_1 + \gamma|u_1| + \gamma|u_2|.
\end{align*}
which finishes the proof.
\end{proof}

\begin{lemma}\label{lem:memory}
After each iteration we have 
$$|W^i|\leq L\cdot \frac{\gamma}{1-\gamma}$$
and 
$$|W_b^i|\leq L\cdot \frac{\gamma}{1-\gamma}.$$

\end{lemma}
\begin{proof}
We prove this by induction on $i$. The proof is similar for $W_i$ and $W^i_b$ so we only prove it for $W^i$. For $i=0$ the induction hypothesis is correct. Now assume the hypothesis is correct for round $i-1$, namely
$$|W^{i-1}| \leq L\cdot \frac{\gamma}{1-\gamma}.$$
For round $i$ we have 
\begin{align*}|W^i|&=|W_{i-1} + u_{i-1} -top_k(W_{i-1} + u_{i-1})|\leq \gamma(|W_{i-1} + u_{i-1}|)\leq \gamma( L\cdot \frac{\gamma}{1-\gamma} + L )=  L\cdot \frac{\gamma}{1-\gamma}
\end{align*}
which finishes the proof.
\end{proof}
Now we use the above Lemma to show a recursive relation for the distance between the benign and adversarial models.
\begin{claim}\label{clm:recursive}
We have
\begin{align*}
|M^i - M^i_{b}|_1&\leq|M^{i-1} - M_b^{i-1}|(1 + \frac{2kc_1c_2}{i} )+ L(\frac{c_1|S\setminus S_b|}{i|S|} +\frac{4c_1 \gamma }{i\cdot (1-\gamma)}).
% \stepcounter{equation}\tag{\theequation}\label{eq:006}
\end{align*}
\end{claim}
\begin{proof}
By Lemma \ref{lem:topk} we have,
\begin{align*}
    |top_k(\frac{u_b}{|S_b|} + W_b^{i-1}) - top_k(\frac{u}{|S|} + W^{i-1})|&\leq |(\frac{u_b}{|S_b|} -\frac{u}{|S|})_I| + |(W_b^{i-1} - W^{i-1})|\\
    &~~~+ \gamma \cdot(|\frac{u_b}{|S_b|} + W_b^{i-1}| + |\frac{u}{|S|} + W^{i-1}|).\stepcounter{equation}\tag{\theequation}\label{eq:000}\\
    \end{align*}
    
Now let, $u^*$ be the summation of updates of benign agents on $M^{i}$. Using Lipschitzness of the gradients, we get
\begin{equation}\label{eq:001}|\frac{u_b}{|S_b|} - \frac{u^*}{|S_b|}|_\infty \leq c_2|M^i_b - M^i|_1.\end{equation}
which implies

\begin{equation}\label{eq:001}|(\frac{u_b}{|S_b|} - \frac{u^*}{|S_b|})_I|_1 \leq 2c_2k|M^i_b - M^i|_1.\end{equation}

We also have
\begin{equation}\label{eq:0012}|\frac{u}{|S_b|} - \frac{u^*}{|S_b|}|_1 \leq L\frac{|S \setminus S_b|}{|S_b|}.\end{equation}
and 
\begin{equation}\label{eq:0013}|\frac{u}{|S_b|} - \frac{u}{|S|}|_1 \leq |u|_1\cdot \frac{|S\setminus S_b|}{|S||S_b|}= L\cdot \frac{|S\setminus S_b|}{|S_b|}.\end{equation}
Now combining inequalities \eqref{eq:001}, \eqref{eq:0012} and \eqref{eq:0013} we get
\begin{equation}\label{eq:0014}|(\frac{u_b}{|S_b|} -\frac{u}{|S|})_I| \leq 2c_2k|M^i_b - M^i|_1 + 2L\frac{|S\setminus S_b|}{|S_b|}.\end{equation}

and by Lemma \ref{lem:memory} and the fact that $\frac{u_b}{|S_b|}\leq L$ and $\frac{u}{|S|}\leq L$ we have

\begin{equation}\label{eq:002}|\frac{u_b}{|S_b|}+W_b^{i-1}| \leq \frac{L}{1-\gamma}~~\text{ and } ~~|W_b^{i-1}|\leq \frac{L\gamma}{1-\gamma}.\end{equation}
And similarly, we  
\begin{equation}\label{eq:003}
   \frac{u}{|S|}+W^{i-1}| \leq \frac{L}{1-\gamma}~~\text{ and } ~~|W^{i-1}|\leq \frac{L\gamma}{1-\gamma}.\end{equation}

Therefore combining Inequalities \eqref{eq:000}, \eqref{eq:0014}, \eqref{eq:002} and \eqref{eq:003}
we have
\begin{align*}
    |top_k(\frac{u_b}{|S_b|} + W_b^{i-1}) - top_k(\frac{u}{|S|} + W^{i-1})|\leq 2k\cdot c_2|(M^{i-1}_b - M^{i-1})|_1 + 2\frac{|S\setminus S_b|}{|S|}L +4\frac{\gamma |L|}{1-\gamma} 
    \end{align*}
    
Now using the Lipschitzness of the aggregation algorithm we have
\begin{align*}
|M^i - M^b_{i}|_1&\leq
|M^{i-1} - M_b^{i-1}|
+ \frac{c_1}{i}|top_k(\frac{u_b}{|S_b|} + W_b^{i-1})- top_k(\frac{u}{|S|} + W^{i-1})|\\
&\leq  |M^{i-1} - M_b^{i-1}| + 2k\cdot \frac{c_1}{i} \cdot c_2 |M^{i-1} - M_b^{i-1}|_1 + \frac{c_1}{i}\frac{|S\setminus S_b|}{|S|}L+ \frac{4c_1 \gamma L}{i\cdot (1-\gamma)}
\end{align*}
which finishes the proof.
\end{proof}
The inequality of Claim \ref{clm:recursive} shows a recursive relation between $|M^i - M^i_b|$ and $|M^{i-1}  - M^{i-1}_b|$. The following lemma shows how we can use this recursive relationship to bound the distance. 

\begin{lemma}\label{lem:recursive}
Let $S_{\N}$ be a sequence such that $S_0=0$ 
$$S_{i} \leq (1+A\lambda(i))S_{i-1} + B\lambda(i)$$ for positive $\lembda(i)$
and let $\Lambda(i)=\sum_{j=1}^i \lambda(i)$, then for any $T$ we have
$$S_T \leq \Lambda(i)\cdot (A+1)^{\Lambda(i)}\cdot B.$$
\end{lemma}

\begin{proof}
We prove this by strong induction. Let $P_{\N}$ be a series where $P_i = (\sum_{j=1}^i {1/j}) -1 $. We make the following strong induction hypothesis:
$$S_T \leq (P_T + 1)(1+A)^{P_T}\cdot B$$
Note that this is stronger than our lemma as we have $P_T \leq \ln(T)$. The induction hypothesis is correct for $T=1$. Suppose for $T=i$ we have
$$S_i \leq (P_i + 1)(1+A)^{P_i}\cdot B$$
then, we have
\begin{align*}
    S_{i+1} &\leq (1+\frac{A}{i+1})S_i + \frac{B}{i+1}\\
    &\leq B((1+P_i)(1+A)^{P_i}(1+\frac{A}{i+1}) + \frac{1}{i+1})\\
    \text{(By Bernouli)~}&\leq B((1+P_i)(1+A)^{P_i+ \frac{1}{i+1}} +\frac{1}{i+1})\\
    &=B((1+P_i)(1+A)^{P_{i+1}} +\frac{1}{i+1})\\
    &\leq B((1+P_i)(1+A)^{P_{i+1}}  + \frac{1}{i+1}(1+A)^{P_{i+1}})\\
    &= B(1+P_{i+1})(1+A)^{P_{i+1}}.
\end{align*}
Therefore, the induction hypothesis is correct and the proof is complete.
\end{proof}

Now using the recursive relation of Claim \ref{clm:recursive} and using the fact that $|M^0-M_b^0|=0$ and deploying Lemma \ref{lem:recursive} we get
\begin{align*}|M^{T} - M_b^{T}|&\leq 2c_1L(1+\ln(T)) \cdot (1+ 2k c_1 c_2)^ {\ln(T)}(\frac{|S\setminus S_b|}{|S|} + \frac{2\gamma}{1-\gamma} )\\
&= \tilde{O}(T^{2kc_1c_2}(\frac{|S\setminus S_b|}{|S|} + \frac{2\gamma}{1-\gamma}))
\end{align*}
which finishes the proof.
\end{proof}
\paragraph{Proof of Theorem \ref{thm:inf1} and Theorem \ref{thm:main}:}
Observe that using Theorem \ref{thm:main2} we can directly get Theorem \ref{thm:main}. Also, by setting $k=d$ in Theorem \ref{thm:main2} we get Theorem \ref{thm:inf1}.
% \subsection{Another analysis} The bound we proved in previous section could suffer from polynomial relation with $T$. Although in practice $T$ is much smaller than the dimension $d$, it will still be good to have a bound that has logarithmic relation with $T$ for cases were $T$ can grow significantly. Here, we present another analisys that depends only on $\ln(T)$.
% \begin{theorem}
% With the same conditions as of Theorem \ref{thm:main} we have:

% \begin{align*}&|M^{T} - M_b^{T}|_1\leq\\
% &~~~2c_1L(1+\ln(T)) \cdot (k c_2 \ln(eT) + \frac{|S\setminus S_b|}{|S|} + \frac{2\gamma}{1-\gamma} )
% \end{align*}
% \end{theorem}
