# Supplementary material for: SparseFed: Mitigating Model Poisoning Attacks in Federated Learning with Sparsification
Source: arXiv:2112.06274 source file (2021-12-12)
Supplement: Supplementary file 5 [file proof.tex]

\vspace*{-13pt}
\section{Proof of certification}

% \subsection{Proof of Theorem \ref{thm:main}}
Here, we prove Theorem \ref{}.
Now we are ready to prove Theorem \ref{}. 
\begin{proof}[Proof of Theorem \ref{}]
We first define two sequence of model $(\theta_b^0, \dots, \theta_b^T)$ and $(\theta^0, \dots, \theta^T)$ where $\theta_b^i$ is the model trained in the first $i$ iterations from the benign rule and $\theta^i$ is the model trained in the first $i$ iterations from the adversarial rule. 
% We prove the Theorem by using a series of Lemmas.
% First note that $M_b^0=M^0$ as the first element of the sequence is just the random initialization and is the same for both sequences. Now we make this strong induction hypothesis: At each iteration $i$, we have
% \begin{equation}|W_b^i-W^{i}|+|M^i_b-M^i|_1\leq (1+c_1+c_2)\cdot k \cdot i \cdot L\cdot(\gamma + \frac{|S\setminusS_b|}{|S|})\end{equation}
% Let $W^i$ be the ``memory'' of the top-$k$ at iteration $i$ and $W^i_b$ be the memory when only the gradients of the benign agents are used up to iteration $i$. 
% Note that the hypothesis is correct for $i=0$. Now assume we assume the hypothesis for $i-1$ and prove it for $i$. Assume we have
% \begin{equation}|W_b^{i-1}-W^{i-1}|+|M^i_b-M^i|_1\leq (1+c_1+c_2)\cdot k \cdot (i-1) \cdot L\cdot(\gamma + \frac{|S\setminusS_b|}{|S|}).\end{equation}

Let $u$ be the output update vector of the adversarial rule and $u_b$  update vector of benign rule. By definition of $\gamma$ we have
$$|top_k(u_b) -top_k(u)|\leq \rho + \gamma.$$


Now we show a recursive relation for the distance between the benign and adversarial models.
\begin{claim}\label{clm:recursive}
We have
\begin{align*}
|\theta^i - \theta^i_{b}|_1&\leq|\theta^{i-1} - \theta_b^{i-1}|(1 + 2kc\lambda(t) )+ (\rho + \gamma)\cdot \lambda(t) .
% \stepcounter{equation}\tag{\theequation}\label{eq:006}
\end{align*}
\end{claim}
\begin{proof}
Let $I=$We have,
\begin{align*}
    |top_k(u_b) - top_k(u)|&\leq |(\frac{u_b}{|S_b|} -\frac{u}{|S|})_I| + |(W_b^{i-1} - W^{i-1})|\\
    &~~~+ \gamma \cdot(|\frac{u_b}{|S_b|} + W_b^{i-1}| + |\frac{u}{|S|} + W^{i-1}|).\stepcounter{equation}\tag{\theequation}\label{eq:000}\\
    \end{align*}
    
Now let, $u^*=\cA_\epsilon(\cG(\cL(\theta_i,D)))$ be the output gradient  of the adversarial rule on $\theta{i}$. Also, let $u_b$ be the 
Using coordinatewise Lipschitzness of the gradients, we get
\begin{equation}\label{eq:001}|u_b -u^*|_\infty \leq c|\theta^i_b - \theta^i|_1.\end{equation}
which implies

\begin{equation}\label{eq:001}|(\frac{u_b}{|S_b|} - \frac{u^*}{|S_b|})_I|_1 \leq 2c_2k|\thetai_b - \thetai|_1.\end{equation}

We also have
\begin{equation}\label{eq:0012}|\frac{u}{|S_b|} - \frac{u^*}{|S_b|}|_1 \leq L\frac{|S \setminus S_b|}{|S_b|}.\end{equation}
and 
\begin{equation}\label{eq:0013}|\frac{u}{|S_b|} - \frac{u}{|S|}|_1 \leq |u|_1\cdot \frac{|S\setminus S_b|}{|S||S_b|}= L\cdot \frac{|S\setminus S_b|}{|S_b|}.\end{equation}
Now combining inequalities \eqref{eq:001}, \eqref{eq:0012} and \eqref{eq:0013} we get
\begin{equation}\label{eq:0014}|(\frac{u_b}{|S_b|} -\frac{u}{|S|})_I| \leq 2c_2k|\thetai_b - \thetai|_1 + 2L\frac{|S\setminus S_b|}{|S_b|}.\end{equation}

and by Lemma \ref{lem:memory} and the fact that $\frac{u_b}{|S_b|}\leq L$ and $\frac{u}{|S|}\leq L$ we have

\begin{equation}\label{eq:002}|\frac{u_b}{|S_b|}+W_b^{i-1}| \leq \frac{L}{1-\gamma}~~\text{ and } ~~|W_b^{i-1}|\leq \frac{L\gamma}{1-\gamma}.\end{equation}
And similarly, we  
\begin{equation}\label{eq:003}
   \frac{u}{|S|}+W^{i-1}| \leq \frac{L}{1-\gamma}~~\text{ and } ~~|W^{i-1}|\leq \frac{L\gamma}{1-\gamma}.\end{equation}

Therefore combining Inequalities \eqref{eq:000}, \eqref{eq:0014}, \eqref{eq:002} and \eqref{eq:003}
we have
\begin{align*}
    |top_k(\frac{u_b}{|S_b|} + W_b^{i-1}) - top_k(\frac{u}{|S|} + W^{i-1})|\leq 2k\cdot c_2|(\theta{i-1}_b - \theta{i-1})|_1 + 2\frac{|S\setminus S_b|}{|S|}L +4\frac{\gamma |L|}{1-\gamma} 
    \end{align*}
    
Now using the Lipschitzness of the aggregation algorithm we have
\begin{align*}
|\thetai - \thetab_{i}|_1&\leq
|\theta{i-1} - M_b^{i-1}|
+ \frac{c_1}{i}|top_k(\frac{u_b}{|S_b|} + W_b^{i-1})- top_k(\frac{u}{|S|} + W^{i-1})|\\
&\leq  |\theta{i-1} - M_b^{i-1}| + 2k\cdot \frac{c_1}{i} \cdot c_2 |\theta{i-1} - M_b^{i-1}|_1 + \frac{c_1}{i}\frac{|S\setminus S_b|}{|S|}L+ \frac{4c_1 \gamma L}{i\cdot (1-\gamma)}
\end{align*}
which finishes the proof.
\end{proof}
The inequality of Claim \ref{clm:recursive} shows a recursive relation between $|\thetai - \thetai_b|$ and $|\theta{i-1}  - \theta{i-1}_b|$. The following lemma shows how we can use this recursive relationship to bound the distance. 

\begin{lemma}\label{lem:recursive}
Let $S_{\N}$ be a sequence such that $S_0=0$ 
$$S_{i} \leq (1+\frac{A}{i})S_{i-1} + \frac{B}{i}$$
then for any $T$ we have
$$S_T \leq (1+\ln(T))\cdot {(A+1)^{\ln(T)}}\cdot B.$$
\end{lemma}

\begin{proof}
We prove this by strong induction. Let $P_{\N}$ be a series where $P_i = (\sum_{j=1}^i {1/j}) -1 $. We make the following strong induction hypothesis:
$$S_T \leq (P_T + 1)(1+A)^{P_T}\cdot B$$
Note that this is stronger than our lemma as we have $P_T \leq \ln(T)$. The induction hypothesis is correct for $T=1$. Suppose for $T=i$ we have
$$S_i \leq (P_i + 1)(1+A)^{P_i}\cdot B$$
then, we have
\begin{align*}
    S_{i+1} &\leq (1+\frac{A}{i+1})S_i + \frac{B}{i+1}\\
    &\leq B((1+P_i)(1+A)^{P_i}(1+\frac{A}{i+1}) + \frac{1}{i+1})\\
    \text{(By Bernouli)~}&\leq B((1+P_i)(1+A)^{P_i+ \frac{1}{i+1}} +\frac{1}{i+1})\\
    &=B((1+P_i)(1+A)^{P_{i+1}} +\frac{1}{i+1})\\
    &\leq B((1+P_i)(1+A)^{P_{i+1}}  + \frac{1}{i+1}(1+A)^{P_{i+1}})\\
    &= B(1+P_{i+1})(1+A)^{P_{i+1}}.
\end{align*}
Therefore, the induction hypothesis is correct and the proof is complete.
\end{proof}

Now using the recursive relation of Claim \ref{clm:recursive} and using the fact that $|\theta0-M_b^0|=0$ and deploying Lemma \ref{lem:recursive} we get
\begin{align*}|\theta{T} - M_b^{T}|&\leq 2c_1L(1+\ln(T)) \cdot (1+ 2k c_1 c_2)^ {\ln(T)}(\frac{|S\setminus S_b|}{|S|} + \frac{2\gamma}{1-\gamma} )\\
&= \tilde{O}(T^{2kc_1c_2}(\frac{|S\setminus S_b|}{|S|} + \frac{2\gamma}{1-\gamma}))
\end{align*}
which finishes the proof.
\end{proof}
\paragraph{Proof of Theorem \ref{thm:inf1} and Theorem \ref{thm:main}:}
Observe that using Theorem \ref{thm:main2} we can directly get Theorem \ref{thm:main}. Also, by setting $k=d$ in Theorem \ref{thm:main2} we get Theorem \ref{thm:inf1}.
% \subsection{Another analysis} The bound we proved in previous section could suffer from polynomial relation with $T$. Although in practice $T$ is much smaller than the dimension $d$, it will still be good to have a bound that has logarithmic relation with $T$ for cases were $T$ can grow significantly. Here, we present another analisys that depends only on $\ln(T)$.
% \begin{theorem}
% With the same conditions as of Theorem \ref{thm:main} we have:

% \begin{align*}&|\theta{T} - M_b^{T}|_1\leq\\
% &~~~2c_1L(1+\ln(T)) \cdot (k c_2 \ln(eT) + \frac{|S\setminus S_b|}{|S|} + \frac{2\gamma}{1-\gamma} )
% \end{align*}
% \end{theorem}


% \label{appendix:theory}
% \begin{definition}
% For a parameter $1 \leq k \leq d$, the operator $top_k$: $\mathbb{R}^d \rightarrow \mathbb{R}^d$ is defined for $x \in \mathbb{R}^d$ as
% % \begin{center}
% %\vspace*{-5pt}
% % \begin{align}
% $
%     (\text{top-}k(x))_i \coloneqq \begin{cases}
%     (x)_\pi(i) & \text{if $i \leq k$}\\
%     0 & \text{otherwise}
%     \end{cases}
%     $
    
% % \end{align}
% % \end{center}
% where $\pi$ is a permutation of $[d]$ such that $(|x|)_{\pi}(i) \geq (|x|)_{\pi}(i+1)$ for $i=1,..., d-1$. 
% \end{definition}
% \vspace*{-5pt}

% \paragraph{Robustness of norm clipping:}
% We begin by analyzing the $\ell_2$ clipping component of \algoname{} in isolation without top-$k$, and see that we need further defenses to mitigate the model poisoning attack.
% % \prateek{should we rephrase this text to highlight that we are analyzing the norm clipping component of our defense in isolation here, without top-k?}
% % Our key insight is to combine global top-$k$ update sparsification with norm clipping as a defense mechanism.
% We aim to calculate an upper bound on the distance between attacked and unattacked models trained with federated learning.
% % Federated learning consists of multiple rounds; at each round, a a subset of devices sends an update that is taken with respect to the current model, that is the summary of the protocol so far.
% % As we mention in Section \ref{sec: related_work}, making updates differentially private can mitigate the impact of attackers.
% % Because boosting is typically necessary in order to ensure the attacker can insert their backdoor, $\ell_2$ norm clipping introduces robustness by diminishing the effect of boosting.
% % Afterwards, a Lipschitz mechanism such as uniform averaging combines the gradients and updates the model.
% We first bound the update of iteration $i$ for a federated learning system that implements $\ell_2$ clipping of norm $L$ as:
% \[|u^i-u^i_b|_1 \leq \sqrt{d}L\cdot p.\]
% where $u^i$ is the gradient aggregated over all users, $u^i_b$ is the gradient aggregated over only benign parties, and $p$ is the fraction of attackers in the population.
% If the protocol only has 1 round where attackers may be present, norm clipping will be sufficient to mitigate their effects.
% However, the protocol has multiple adaptive rounds, and any small change in iteration $i$ can propagate and lead to large changes in the next iterations.
% To handle this propagation error, we need to bound the effect that changes in previous rounds have on the gradients of future rounds. 
% This is where we employ our Lipschitzness guarantees. 
% We prove the following informal theorem that uses the Lipschitz continuity of the gradients:
% \begin{theorem}[Robustness of $L_2$ norm clipping]\label{thm:inf1}
% For a protocol with $c$-Lipschitz coordinate-wise gradients, using $\ell_2$ norm clipping with threshold $L$ and decreasing learning rate $\frac{\alpha}{i}$ we have
% %\vspace*{-10pt}
% $$|M^T -M^T_b|_1\leq \tilde{O}(\alpha T^{\alpha d c}Lp\sqrt{d})$$
% where $d$ is the dimension of the model $M$, $p$ is the fraction of corrupted devices, $M^T$ is the model obtained after $T$ iterations and $M^T_b$ is the model after $T$ iterations using only benign devices.
% \end{theorem}

% \paragraph{Robustness of \algoname{}:} In practice $d$ is large, therefore $\ell_2$ clipping is insufficient to mitigate attacks.
% We confirm this analysis with our experiments in Section \ref{sec: evaluation}.
% Next we show that the combination of gradient sparsification and $\ell_2$ clipping can alleviate the curse of dimensionality, and obtain better robustness guarantees.
% % \begin{definition}[ $top_k$ with memory and $\gamma_k$]\label{def:gamma}
% % We can apply the $top_k$ operator to any aggregator $A$ to obtain a new aggregator $A^k$: $A^k$ initializes a memory vector $W_0=0^d$ and an initialization $M_0$.
% % At step $i$, $A^k$ receives the update $u^1,\dots,u^n$ and calculates the $top_k$ $I=\set{i\in [d]; top_k(W_{i-1}+\sum_{j=1}^nu^j)\neq 0}$.
% % Then, the memory and model are updated:
% % %\vspace*{-5pt} % ICML
% % {\begin{small}
% % \begin{align}
% % W_i = W_{i-1} +\sum_{j=1}^nu^j - top_k(W_{i-1}+\sum_{j=1}^n(u^j))
% % M_i=A_i(M_{i-1}, (u^1)_I,\dots,(u^n)_I) 
% % \end{align}
% % \end{small}}
% % %\vspace*{-2pt} % ICML
% % where $(u)_I$ is a vector that is $0$ everywhere except on coordinates $i\in I$ where it is equal to $u$.
% % We also define $\gamma_k$ to be the fraction of $l_1$ mass of information lost via $top_k$.
% % Specifically, for any model $M$, any $i\in [T]$ and update vector $(u^1,\dots,u^n)$ calculated by all parties (including attackers), and memory $W$, we have:
% % %\vspace*{-10pt} % ICML
% % \begin{align}
% %     |top_k(\sum_{j=1}^n u^j + W)|_1\geq (1-\gamma_k)|\sum_{j=1}^n u^j +W|_1.
% % \end{align}
% % %\vspace*{-2pt} % ICML
% % When clear from the context, we use $\gamma$ instead of $\gamma_k$. Note that $\gamma_k$ can be a function of the distribution of the updates and $k$. 
% % For example, if the updates are concentrated on a small number of coordinates, we expect $top_k$ to recover nearly the entire mass and $\gamma_k$ to be small. 
% % \end{definition}

% \begin{theorem}\label{thm:main}
% Let $(f,A)$ be a $(c_1,c_2)$-Lipschitz protocol such that $f_i$ uses a learning rate of $\alpha_i$.
% Let $A^{L,k}$ be the the same aggregator as $A$ but equipped with $\ell_2$-norm clipping and with a clipping threshold of $L$, and the $top_k$ operator. 
% Let $M_b$ be the model obtained by learning using the set of benign devices $S_b$, and $M$ be the model obtained by learning using all devices (including attackers) in $T$ iterations using the protocol $(f,A^{L,K})$. 
% Then we have:
% %\vspace*{-5pt} % ICML
% $$|M^T -M^T_b|_1\leq \tilde{O}(\alpha T^{\alpha k c}L\sqrt{d}(p + \gamma_k)).$$
% %\vspace*{-20pt} % ICML
% \end{theorem}
% % Before proving Theorem \ref{thm:main}, we state a Corollary that simplifies this bound. 
% % \begin{corollary}\label{cor:inf}
% % Simplifying the bound of Theorem \ref{thm:main} we get

% % \end{corollary}

% Comparing Theorem \ref{thm:main} above with Theorem \ref{thm:inf1}, we see that we have improved the exponent of $T$ from $cd$ to $ck$.
% $cd$ is the Lipschitz constant of the model when $top_k$ is not deployed, which we reduce it to $ck$ by using $top_k$ operator.
% This bound on how far the attacker can shift the model acts as an additional constraint on the attacker, that can only improve security.
% In Appendix B.6 we confirm that reducing the distance improves robustness.

% This improvement does not come for free. 
% In general, $\gamma_k$ is an decreasing function of $k$, however, our experiments show that we can obtain very small values of $\gamma_k$ with $k<<d$. 
% Another important consideration is the number of iterations.
% When $k$ is very small, we expect the number of iterations required for convergence to increase. 
% % \prateek{seems important to show this degradation of convergence with k in our results? Ashwinee: it's in Figure 1? what else do you think should be there?}
% To optimize this trade-off, in Section \ref{sec: evaluation} we find small values of $k$ that provide us with strong robustness.

% \emph{In summary, our \algoname{} protocol  aggregates $\ell_2$ clipped gradients from devices and only updates the top-$k$ coordinates of the aggregated gradient.
% We show that the use of top-$k$ update sparsification upper bounds the distance that an attacker can shift the model over the course of training.}

% % \prateek{it could be useful to have a summary sentence about our proposed defense (update sparsification/norm clipping) + another one on the L2 distance bound Ashwinee: How's this?}

% % \begin{proof}[Proof of Theorem \ref{thm:main}]
% % We define two sequences of models $(M_b^0, \dots, M_b^T)$ and $(M^0, \dots, M^T)$ where $M_b^i$ is the model trained in the first $i$ iterations from the data of devices in  $S_b$ and $M^i$ is the model trained in the first $i$ iterations for all devices.
% % We prove Theorem \ref{thm:main} with a series of Lemmas.
% % Let $W^i$ be the memory of $top_k$ at iteration $i$ and $W^i_b$ be the memory when only the gradients of the benign devices are used up to iteration $i$. 
% % Let $u$ be the summation of update vectors of all devices on $M^{i-1}$ and $u_b$ the summation of update vectors of benign devices in $S_b$ over $M^{i-1}_b$. 
% % We first want to bound
% % $$|top_k(\frac{u_b}{|S_b|} + W_b^{i-1}) - top_k(\frac{u}{|S|} + W^{i-1})|.$$

% % We first state the following claim
% % that shows a recursive relationship for the distance between the benign and adversarial models. 
% % The proof of this claim is deferred to the Appendix.
% % \begin{claim}\label{clm:recursive}
% % We have
% % \begin{align*}
% % |M^i - M^i_{b}|_1&\leq|M^{i-1} - M_b^{i-1}|(1 + \frac{2kc_1c_2}{i} )\\
% %  &~~~+ L\sqrt{d}(\frac{c_1|S\setminus S_b|}{i|S|} +\frac{4c_1 \gamma }{i\cdot (1-\gamma)}).
% % % \stepcounter{equation}\tag{\theequation}\label{eq:006}
% % \end{align*}
% % \end{claim}
% % The inequality of Claim \ref{clm:recursive} shows a recursive relation between $|M^i - M^i_b|$ and $|M^{i-1}  - M^{i-1}_b|$. The following lemma shows how we can use this recursive relationship to bound the distance.
% % \begin{lemma}\label{lem:recursive}
% % Let $S_{\N}$ be a sequence such that $S_0=0$ 
% % $$S_{i} \leq (1+\frac{A}{i})S_{i-1} + \frac{B}{i}$$
% % then for any $T$ we have
% % $$S_T \leq (1+\ln(T))\cdot {(A+1)^{\ln(T)}}\cdot B.$$
% % \end{lemma}
% % Now using the recursive relation of Claim \ref{clm:recursive} and using the fact that $|M^0-M_b^0|=0$ and deploying Lemma \ref{lem:recursive} we get
% % \begin{align*}&|M^{T} - M_b^{T}|\leq\\
% % &c_1L\sqrt{d}(1+\ln(T)) \cdot (2+ 4k c_1 c_2)^ {\ln(T)}(\frac{|S\setminus S_b|}{|S|} + \frac{2\gamma}{1-\gamma} )
% % \end{align*}
% % which finishes the proof.
% % \end{proof}

% % Federated learning is a protocol consisting of $n$ parties $P_1,\dots,P_n$ and a central aggregator $G$. 
% \begin{definition}[Federated Learning Protocol] Considering a federated learning protocol with $n$ clients $P_1,\dots,P_n$.
% Let $Z$ be the data domain and ${\cP_i}_{i=1}^{n}$ be $n$ probability distributions over $Z$.
% The $i^{th}$ client has a dataset $D_i$ drawn i.i.d. from $\cP_i$.
% % Let $\cM$ be the class of models in $d$ dimensions, and $\cL: \cM \times Z \rightarrow \cR$ be a loss function.
% % Our goal is to minimize the empirical risk:
% % \begin{align}
% %     f(\M) = \hat{\mathbb{E}}f_i(\M) =
% %     \frac{1}{n}\sum_{i=1}^n \Eu{\z \sim \cP_i}\cL(\M,\z).
% % \end{align}
% We conduct $T$ rounds of the protocol, and at round $i\in[T]$ each participating client downloads the current model $M_{i-1}$.
% % Each $P_i$ has a dataset $D_i$. The aggregator $G$ holds an initial model $M_0$. The protocol consists of $T$ rounds and at round $i\in [T]$, the aggregator sends $M_{i-1}$ to all parties. 
% % Each of them calculate a (potentially randomized) function $f_i$ on their data
% % $$u^j_i=f_i(M_{i-1}, D_j)$$
% % and send it back to the aggregator. Then the aggregator applies a function $A$ to aggregate all the updates

% % $$M_i=A_i(M_{i-1}, u_i^1,\dots,u^n_i).$$

% % For instance, if the goal of this protocol is to train a network using SGD with simple averaging aggregation, then 
% For example, one common instantiation of a federated learning protocol is the following: Each client calculates the result of gradient descent $f_i$ on its data:

% $$f_i(\M, D) =  \frac{\partial \cL(\M,D)}{\partial \M}$$

% And the parameter server averages the updates across participating clients:

% $$A_i(M_{i-1}, u_i^1,\dots,u^n_i) = M_{i-1} + \frac{1}{n}\sum_{j=1}^n u_i^j$$
% \end{definition}
% %  where $\beta_i$ could be seen as the decaying learning rate and is usually set to $\frac{\alpha}{i}$ for some constant $\alpha$.
% \begin{definition}[Lipschitz Federated Learning] A federated learning protocol is $(c_1,c_2)$-Lipschitz if for any round $i\in[T]$, any two models $M_1, M_2\in \cM$, any two sequences of update vectors $(u^1,\dots,u^n)$ and $(u'^1,\dots,u'^m)$, and any dataset $D$ we have
% $$|f_i(M_2,D)-f_i(M_1,D)|_\infty \leq c_1\cdot |M_2-M_1|_1$$
% and 
% \begin{align*}
%     &|A_i(M_1, u^1,\dots,u^n) - A_i(M_2,u'^1,\dots,u'^m)|_1\leq |M_1-M_2|_1 + \frac{c_2}{i}(|\frac{\sum_{j=1}^{n}u^j}{n}-\frac{\sum_{j=1}^{m}u'^j}{m}|_1)
% \end{align*}
% \end{definition}

% \begin{definition}\label{def:gamma}[$\gamma_k$ for top-$k$ operator]
% Let $\gamma_k$ be the fraction of $l_1$ mass of information lost via $top_k$, where $top_k(u)$ recovers a $1-\gamma_k$ fraction of the $l_1$ mass of $u$.
% % In particular, $1-\gamma_k$ fraction of the $l_1$-norm mass of the gradients should be recovered after top-$k$ is applied. 
% For any model $M$, any $i\in [T]$ and update vector $(u^1,\dots,u^n)$ calculated by all parties (including benign and adversarial gradients), and memory $W$, we have:
% \begin{align}
%     |top_k(\sum_{j=1}^n u^j + W)|_1\geq (1-\gamma_k)|\sum_{j=1}^n u^j +W|_1.
% \end{align}
% When clear from the context, we use $\gamma$ instead of $\gamma_k$.
% \end{definition}
% Now we prove the following general Theorem that we use to prove Theorems \ref{thm:inf1} and \ref{thm:main}.
% \begin{theorem}\label{thm:main2}
% Let $(f,A)$ be a $(c_1,c_2)$-Lipschitz protocol such that $f_i$ uses a learning rate of $\alpha_i$.
% Let $A_{L,k}$ be the aggregator that conducts an average, equipped with $l_1$-norm clipping with a clipping threshold of $L$, and the top-$k$ operator. 
% Let $M_b$ be the model obtained by learning using the set of benign agents $S_b$, and $M$ be the model obtained by learning using all agents (benign and adversarial) in $T$ iterations using the protocol $(f,A_{L,K})$. 
% Then we have:

% \begin{align*}&|M^{T} - M_b^{T}|_1\leq2c_1L(1+\ln(T)) \cdot (1+ 2k c_1 c_2)^ {\ln(T)}(\frac{|S\setminus S_b|}{|S|} + \frac{2\gamma}{1-\gamma} =\tilde{O}(\alpha T^{2k c_1c_2}L\sqrt{d}(p + \gamma_k)).)
% \end{align*}
% \end{theorem}
% \begin{proof}
% We first define two sequence of model $(M_b^0, \dots, M_b^T)$ and $(M^0, \dots, M^T)$ where $M_b^i$ is the model trained in the first $i$ iterations from the data of the agents in  $S_b$ and $M^i$ is the model trained in the first $i$ iterations for all agents.  We prove the Theorem by using a series of Lemmas.
% % First note that $M_b^0=M^0$ as the first element of the sequence is just the random initialization and is the same for both sequences. Now we make this strong induction hypothesis: At each iteration $i$, we have
% % \begin{equation}|W_b^i-W^{i}|+|M^i_b-M^i|_1\leq (1+c_1+c_2)\cdot k \cdot i \cdot L\cdot(\gamma + \frac{|S\setminusS_b|}{|S|})\end{equation}
% Let $W^i$ be the ``memory'' of the top-$k$ at iteration $i$ and $W^i_b$ be the memory when only the gradients of the benign agents are used up to iteration $i$. 
% % Note that the hypothesis is correct for $i=0$. Now assume we assume the hypothesis for $i-1$ and prove it for $i$. Assume we have
% % \begin{equation}|W_b^{i-1}-W^{i-1}|+|M^i_b-M^i|_1\leq (1+c_1+c_2)\cdot k \cdot (i-1) \cdot L\cdot(\gamma + \frac{|S\setminusS_b|}{|S|}).\end{equation}

% Let $u$ be the summation of update vectors of all agents on $M^{i-1}$ and $u_b$ the summation of update vector of benign agents in $S_b$ over $M^{i-1}_b$. We first want to bound
% $$|top_k(\frac{u_b}{|S_b|} + W_b^{i-1}) - top_k(\frac{u}{|S|} + W^{i-1})|.$$

% For that, we first prove the following two Lemmas whose proofs are deferred to appendix. 

% \begin{lemma}\label{lem:topk}
% Let $u_1$ and $u_2$ be two vectors in $\mathbb{R}^d$ such that $|top_k(u_1)|\geq(1-\gamma)\cdot |u_1|$ and  $|top_k(u_2)|\geq(1-\gamma)\cdot |u_2|$, then, for any vector $v$ we have
% \begin{align*}
%     &|top_k(u_1)-top_k(u_2)|_1 \leq |(u_1-u_2)_I|_1 + 2\gamma |u_2|_1 + 2\gamma |u_1|_1 
% \end{align*}
% where $I=\set{j\in [d] \text{~s.t.~} top_k(u_1)[j]\neq 0 \text{~or~}  top_k(u_2)[j]\neq 0}$.

% \end{lemma}

% \begin{proof}
% Let $\tau_1$ and $\tau_2$ be two vectors such that $\tau_1[i]=1$ if $top_k(u_1)[i]\neq0$ and $\tau_1[i]=0$ otherwise. Similarly, $\tau_2[i]=1$ if $top_k(u_2)[i]\neq0$ and  $\tau_2[i]=0$ otherwise. Let $I'$ be the locations where $\tau_1[i]=1$ and $\tau_2[i]=1$. Now we have

% \begin{align*}
%     |top_k(u_1) -top_k(u_2)|
%     &= \sum_{i=1}^d |u_1[i]\tau_1[i] - u_2[i]\tau_2[i]| \\
%     &= |(u_1-u_2)_{I'}|_1 + \sum_{i\in I\setminus I' } |u_1[i]\tau_1[i] - u_2[i]\tau_2[i]|\\
%     &\leq |(u_1-u_2)_{I'}|_1 + \sum_{i \in I\setminus I' } |u_1[i]\tau_1[i] - u_2[i]\tau_1[i]|\\
%     &~~+\sum_{i \in I\setminus I' }|u_1[i]\tau_2[i] - u_2[i]\tau_2[i]|+ \sum_{i \in I\setminus I' }|u_2[i]\tau_1[i] - u_1[i]\tau_2[i] |\\
%     &= |(u_1-u_2)_I|_1+ \sum_{i \in I\setminus I' }|u_2[i]\tau_1[i] - u_1[i]\tau_2[i] |\\
%     &\leq |(u_1-u_2)_I|_1 + \sum_{i\in I\setminus I' } |u_1[i]\tau_2[i]| + |u_2[i]\tau_1[i]|\\
%     &= |(u_1-u_2)_I|_1 + \sum_{i\in I\setminus I' } |u_1[i](1-\tau_1[i])|+ \sum_{i\in I\setminus I' } |u_2[i](1-\tau_2[i])|\\
%     &\leq |(u_1-u_2)_I|_1 +  |u_1 -top_k(u_1)| + |u_2-top_k(u_2)|\\
%     &\leq |(u_1-u_2)_I|_1 + \gamma|u_1| + \gamma|u_2|.
% \end{align*}
% which finishes the proof.
% \end{proof}

% \begin{lemma}\label{lem:memory}
% After each iteration we have 
% $$|W^i|\leq L\cdot \frac{\gamma}{1-\gamma}$$
% and 
% $$|W_b^i|\leq L\cdot \frac{\gamma}{1-\gamma}.$$

% \end{lemma}
% \begin{proof}
% We prove this by induction on $i$. The proof is similar for $W_i$ and $W^i_b$ so we only prove it for $W^i$. For $i=0$ the induction hypothesis is correct. Now assume the hypothesis is correct for round $i-1$, namely
% $$|W^{i-1}| \leq L\cdot \frac{\gamma}{1-\gamma}.$$
% For round $i$ we have 
% \begin{align*}|W^i|&=|W_{i-1} + u_{i-1} -top_k(W_{i-1} + u_{i-1})|\leq \gamma(|W_{i-1} + u_{i-1}|)\leq \gamma( L\cdot \frac{\gamma}{1-\gamma} + L )=  L\cdot \frac{\gamma}{1-\gamma}
% \end{align*}
% which finishes the proof.
% \end{proof}
% Now we use the above Lemma to show a recursive relation for the distance between the benign and adversarial models.
% \begin{claim}\label{clm:recursive}
% We have
% \begin{align*}
% |M^i - M^i_{b}|_1&\leq|M^{i-1} - M_b^{i-1}|(1 + \frac{2kc_1c_2}{i} )+ L(\frac{c_1|S\setminus S_b|}{i|S|} +\frac{4c_1 \gamma }{i\cdot (1-\gamma)}).
% % \stepcounter{equation}\tag{\theequation}\label{eq:006}
% \end{align*}
% \end{claim}
% \begin{proof}
% By Lemma \ref{lem:topk} we have,
% \begin{align*}
%     |top_k(\frac{u_b}{|S_b|} + W_b^{i-1}) - top_k(\frac{u}{|S|} + W^{i-1})|&\leq |(\frac{u_b}{|S_b|} -\frac{u}{|S|})_I| + |(W_b^{i-1} - W^{i-1})|\\
%     &~~~+ \gamma \cdot(|\frac{u_b}{|S_b|} + W_b^{i-1}| + |\frac{u}{|S|} + W^{i-1}|).\stepcounter{equation}\tag{\theequation}\label{eq:000}\\
%     \end{align*}
    
% Now let, $u^*$ be the summation of updates of benign agents on $M^{i}$. Using Lipschitzness of the gradients, we get
% \begin{equation}\label{eq:001}|\frac{u_b}{|S_b|} - \frac{u^*}{|S_b|}|_\infty \leq c_2|M^i_b - M^i|_1.\end{equation}
% which implies

% \begin{equation}\label{eq:001}|(\frac{u_b}{|S_b|} - \frac{u^*}{|S_b|})_I|_1 \leq 2c_2k|M^i_b - M^i|_1.\end{equation}

% We also have
% \begin{equation}\label{eq:0012}|\frac{u}{|S_b|} - \frac{u^*}{|S_b|}|_1 \leq L\frac{|S \setminus S_b|}{|S_b|}.\end{equation}
% and 
% \begin{equation}\label{eq:0013}|\frac{u}{|S_b|} - \frac{u}{|S|}|_1 \leq |u|_1\cdot \frac{|S\setminus S_b|}{|S||S_b|}= L\cdot \frac{|S\setminus S_b|}{|S_b|}.\end{equation}
% Now combining inequalities \eqref{eq:001}, \eqref{eq:0012} and \eqref{eq:0013} we get
% \begin{equation}\label{eq:0014}|(\frac{u_b}{|S_b|} -\frac{u}{|S|})_I| \leq 2c_2k|M^i_b - M^i|_1 + 2L\frac{|S\setminus S_b|}{|S_b|}.\end{equation}

% and by Lemma \ref{lem:memory} and the fact that $\frac{u_b}{|S_b|}\leq L$ and $\frac{u}{|S|}\leq L$ we have

% \begin{equation}\label{eq:002}|\frac{u_b}{|S_b|}+W_b^{i-1}| \leq \frac{L}{1-\gamma}~~\text{ and } ~~|W_b^{i-1}|\leq \frac{L\gamma}{1-\gamma}.\end{equation}
% And similarly, we  
% \begin{equation}\label{eq:003}
%   \frac{u}{|S|}+W^{i-1}| \leq \frac{L}{1-\gamma}~~\text{ and } ~~|W^{i-1}|\leq \frac{L\gamma}{1-\gamma}.\end{equation}

% Therefore combining Inequalities \eqref{eq:000}, \eqref{eq:0014}, \eqref{eq:002} and \eqref{eq:003}
% we have
% \begin{align*}
%     |top_k(\frac{u_b}{|S_b|} + W_b^{i-1}) - top_k(\frac{u}{|S|} + W^{i-1})|\leq 2k\cdot c_2|(M^{i-1}_b - M^{i-1})|_1 + 2\frac{|S\setminus S_b|}{|S|}L +4\frac{\gamma |L|}{1-\gamma} 
%     \end{align*}
    
% Now using the Lipschitzness of the aggregation algorithm we have
% \begin{align*}
% |M^i - M^b_{i}|_1&\leq
% |M^{i-1} - M_b^{i-1}|
% + \frac{c_1}{i}|top_k(\frac{u_b}{|S_b|} + W_b^{i-1})- top_k(\frac{u}{|S|} + W^{i-1})|\\
% &\leq  |M^{i-1} - M_b^{i-1}| + 2k\cdot \frac{c_1}{i} \cdot c_2 |M^{i-1} - M_b^{i-1}|_1 + \frac{c_1}{i}\frac{|S\setminus S_b|}{|S|}L+ \frac{4c_1 \gamma L}{i\cdot (1-\gamma)}
% \end{align*}
% which finishes the proof.
% \end{proof}
% The inequality of Claim \ref{clm:recursive} shows a recursive relation between $|M^i - M^i_b|$ and $|M^{i-1}  - M^{i-1}_b|$. The following lemma shows how we can use this recursive relationship to bound the distance. 

% \begin{lemma}\label{lem:recursive}
% Let $S_{\N}$ be a sequence such that $S_0=0$ 
% $$S_{i} \leq (1+\frac{A}{i})S_{i-1} + \frac{B}{i}$$
% then for any $T$ we have
% $$S_T \leq (1+\ln(T))\cdot {(A+1)^{\ln(T)}}\cdot B.$$
% \end{lemma}

% \begin{proof}
% We prove this by strong induction. Let $P_{\N}$ be a series where $P_i = (\sum_{j=1}^i {1/j}) -1 $. We make the following strong induction hypothesis:
% $$S_T \leq (P_T + 1)(1+A)^{P_T}\cdot B$$
% Note that this is stronger than our lemma as we have $P_T \leq \ln(T)$. The induction hypothesis is correct for $T=1$. Suppose for $T=i$ we have
% $$S_i \leq (P_i + 1)(1+A)^{P_i}\cdot B$$
% then, we have
% \begin{align*}
%     S_{i+1} &\leq (1+\frac{A}{i+1})S_i + \frac{B}{i+1}\\
%     &\leq B((1+P_i)(1+A)^{P_i}(1+\frac{A}{i+1}) + \frac{1}{i+1})\\
%     \text{(By Bernouli)~}&\leq B((1+P_i)(1+A)^{P_i+ \frac{1}{i+1}} +\frac{1}{i+1})\\
%     &=B((1+P_i)(1+A)^{P_{i+1}} +\frac{1}{i+1})\\
%     &\leq B((1+P_i)(1+A)^{P_{i+1}}  + \frac{1}{i+1}(1+A)^{P_{i+1}})\\
%     &= B(1+P_{i+1})(1+A)^{P_{i+1}}.
% \end{align*}
% Therefore, the induction hypothesis is correct and the proof is complete.
% \end{proof}

% Now using the recursive relation of Claim \ref{clm:recursive} and using the fact that $|M^0-M_b^0|=0$ and deploying Lemma \ref{lem:recursive} we get
% \begin{align*}|M^{T} - M_b^{T}|&\leq 2c_1L(1+\ln(T)) \cdot (1+ 2k c_1 c_2)^ {\ln(T)}(\frac{|S\setminus S_b|}{|S|} + \frac{2\gamma}{1-\gamma} )\\
% &= \tilde{O}(T^{2kc_1c_2}(\frac{|S\setminus S_b|}{|S|} + \frac{2\gamma}{1-\gamma}))
% \end{align*}
% which finishes the proof.
% \end{proof}
% \paragraph{Proof of Theorem \ref{thm:inf1} and Theorem \ref{thm:main}:}
% Observe that using Theorem \ref{thm:main2} we can directly get Theorem \ref{thm:main}. Also, by setting $k=d$ in Theorem \ref{thm:main2} we get Theorem \ref{thm:inf1}.
% % \subsection{Another analysis} The bound we proved in previous section could suffer from polynomial relation with $T$. Although in practice $T$ is much smaller than the dimension $d$, it will still be good to have a bound that has logarithmic relation with $T$ for cases were $T$ can grow significantly. Here, we present another analisys that depends only on $\ln(T)$.
% % \begin{theorem}
% % With the same conditions as of Theorem \ref{thm:main} we have:

% % \begin{align*}&|M^{T} - M_b^{T}|_1\leq\\
% % &~~~2c_1L(1+\ln(T)) \cdot (k c_2 \ln(eT) + \frac{|S\setminus S_b|}{|S|} + \frac{2\gamma}{1-\gamma} )
% % \end{align*}
% % \end{theorem}
